# Supplementary material for: Real-Time Dispatching of Large-Scale Ride-Sharing Systems: Integrating Optimization, Machine Learning, and Model Predictive Control
Source: arXiv:2003.10942 source file (2020-03-24)
Supplement: Supplementary file 1 [file appendix.tex]

\section{Appendix}
\begin{figure}[!ht]
  \includegraphics[width=\columnwidth]{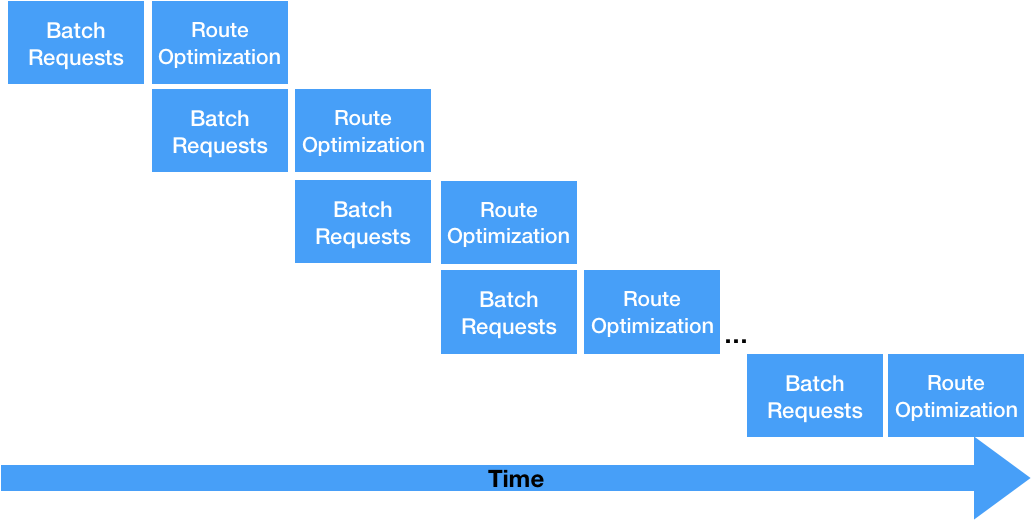}
  \caption{An illustration of the CPAIOR framework.}
  \label{fig:cpaior_framework}
\end{figure}

\begin{figure}
  \includegraphics[width=\columnwidth]{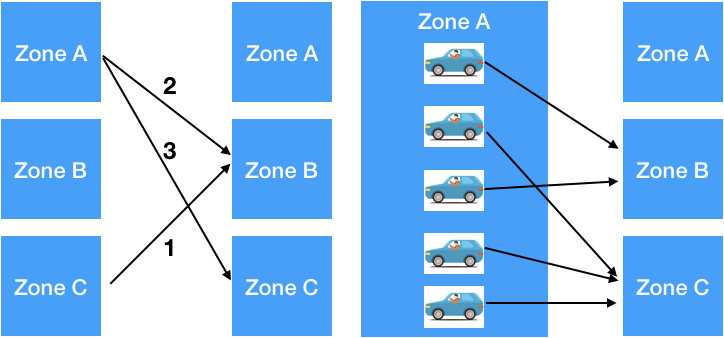}
  \caption{An illustration of the function of the vehicle allocation and vehicle relocation MIPs.}
  \label{fig:va_vr_mip}
\end{figure}
